# Supplementary material for: NeuS: Learning Neural Implicit Surfaces by Volume Rendering for Multi-view Reconstruction
Source: arXiv:2106.10689 source file (2023-02-01)
Supplement: Supplementary file 1 [file bias.tex]

\begin{wrapfigure}{R}{0.4\textwidth}
\centering{
  \includegraphics[width=\linewidth]{supplementary/figure_source/bias.pdf}
  \caption{Illustration of bias in Naive Solution II.}
  \vspace{0pt}
  \label{fig:bias}
}
\end{wrapfigure}
