# Supplementary material for: NeuS: Learning Neural Implicit Surfaces by Volume Rendering for Multi-view Reconstruction
Source: arXiv:2106.10689 source file (2023-02-01)
Supplement: Supplementary file 2 [file compate_thin.tex]

\begin{figure}[!b]
  \includegraphics[width=\linewidth]{supplementary/figure_source/compare_thin.pdf}\\
  \mpage{0.23}{Reference Image}
  \mpage{0.23}{(a) Ours}
  \mpage{0.23}{(b) COLMAP$_{trim=10}$}
  \mpage{0.23}{(c) COLMAP$_{trim=7}$}
  \caption{Qualitative results on the object with thin structures. The left half is the depth map while the right half is the reconstructed surface.}
  \label{fig:thin}
\end{figure}
