# Supplementary material for: NeuS: Learning Neural Implicit Surfaces by Volume Rendering for Multi-view Reconstruction
Source: arXiv:2106.10689 source file (2023-02-01)
Supplement: Supplementary file 4 [file notation.tex]

% notations
