# Supplementary material for: NeuS: Learning Neural Implicit Surfaces by Volume Rendering for Multi-view Reconstruction
Source: arXiv:2106.10689 source file (2023-02-01)
Supplement: Supplementary file 6 [file macro.tex]

%\renewcommand{\baselinestretch}{1}       % for squeezing the draft into the page limit, do not use

% =========================================
% Useful macros
% =========================================

% Latin abbreviations
\def\etal{et al.}			  % and others, and co-workers
\def\eg{e.g.,~}               % for example
\def\ie{i.e.,~}               % that is, in other words
\def\etc{etc}                 % and other things, and so forth
\def\cf{cf.~}                 % compare
\def\viz{viz.~}               % namely, precisely
\def\vs{vs.~}                 % against


% Math related
\DeclareMathOperator*{\argmin}{\arg\!\min} 
\DeclareMathOperator*{\argmax}{\arg\!\max}

% Consistent margin adjustment for paragraphs, figures, and sections
\newlength\paramargin
\newlength\figmargin
\newlength\secmargin
\newlength\figcapmargin

\setlength{\secmargin}{0.0mm}
\setlength{\paramargin}{0.0mm}
\setlength{\figmargin}{0.0mm}
\setlength{\figcapmargin}{0.5mm}

\newcommand{\red}{\textcolor{red}}
\newcommand{\blue}{\textcolor{blue}}

% minipage
\newcommand{\mpage}[2]
{
\begin{minipage}{#1\linewidth}\centering
#2
\end{minipage}
}

\newcommand{\mfigure}[2]
{
\begin{subfigure}[b]{#1\linewidth}\centering
\includegraphics[width=\linewidth]{#2}
\end{subfigure}
}

\newcommand{\Paragraph}[1]
{
\vspace{\paramargin}
\paragraph{#1}
}

\newcommand{\heading}[1]
{
\vspace{1mm}
\noindent \textbf{#1}
}   

% References for figures, tables, equations, and sections
\newcommand{\secref}[1]{Section~\ref{sec:#1}}
\newcommand{\figref}[1]{Figure~\ref{fig:#1}} 
\newcommand{\tblref}[1]{Table~\ref{tbl:#1}}
\newcommand{\eqnref}[1]{Equation~\ref{eq:#1}}
\newcommand{\thmref}[1]{Theorem~\ref{#1}}
\newcommand{\lemmaref}[1]{Lemma~\ref{lemma:#1}}
\newcommand{\prgref}[1]{Program~\ref{#1}}
\newcommand{\algref}[1]{Algorithm~\ref{#1}}
\newcommand{\clmref}[1]{Claim~\ref{#1}}
\newcommand{\lemref}[1]{Lemma~\ref{#1}}
\newcommand{\ptyref}[1]{Property~\ref{#1}}

% Comments
\long\def\ignorethis#1{}
\newcommand {\authorA}[1]{{\color{red}\textbf{AuthorA: }#1}\normalfont}
\newcommand {\authorB}[1]{{\color{magenta}\textbf{AuthorB: }#1}\normalfont}
%\newcommand {\todo}{{\textbf{\color{red}[TO-DO]\_}}}
\newcommand {\todo}[1]{{\textbf{\color{red}[TODO:#1]}}}
\def\newtext#1{\textcolor{blue}{#1}}
\def\modtext#1{\textcolor{red}{#1}}
\newcommand{\note}[1]{{\color{blue} #1}}

\newcommand{\tb}[1]{\textbf{#1}}
\newcommand{\mb}[1]{\mathbf{#1}}
\newcommand{\revised}[1]{\textcolor{red}{#1}}
\newcommand{\hl}[1]{\textcolor{red}{#1}}


\newcommand{\jbox}[2]{
  \fbox{%
  	\begin{minipage}{#1}%
  		\hfill\vspace{#2}%
  	\end{minipage}%
  }}

\newcommand{\jblock}[2]{%
	\begin{minipage}[t]{#1}\vspace{0cm}\centering%
	#2%
	\end{minipage}%
}
